# Supplementary material for: Three-dimensional structure and formation mechanism of biskyrmions in uniaxial ferromagnets
Source: arXiv:2201.06772 source file (2022-01-18)
Supplement: Supplementary file 1 [file supplement.pdf]

## Supplemental Material

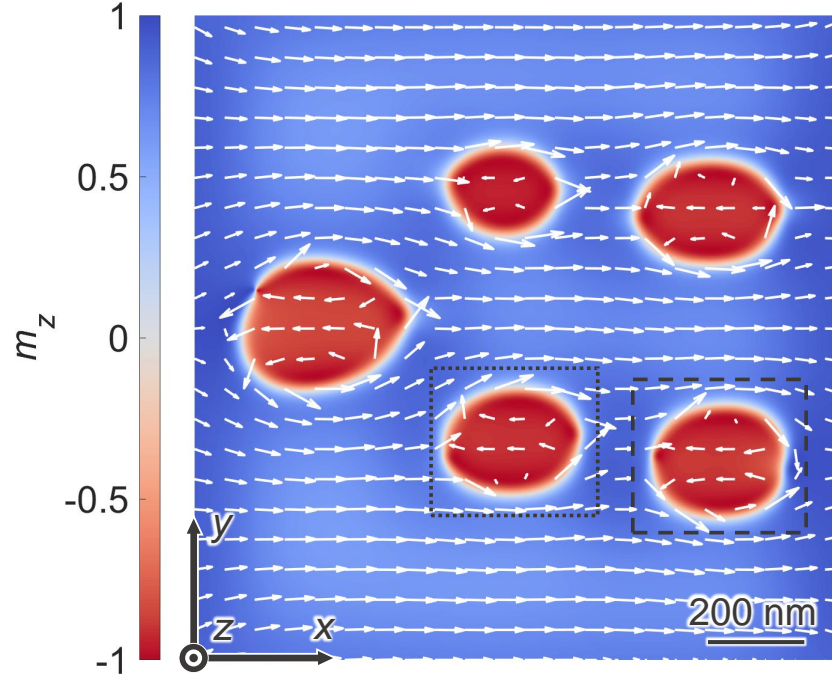

FIG. S1. The complete spin texture in the simulation of Fig.1 in the main text. The biskyrmion in Fig.1(a) of the main text outlined in dash rectangle. The type-II bubble in Fig1.(b) of the main text outlined in dotted rectangle.

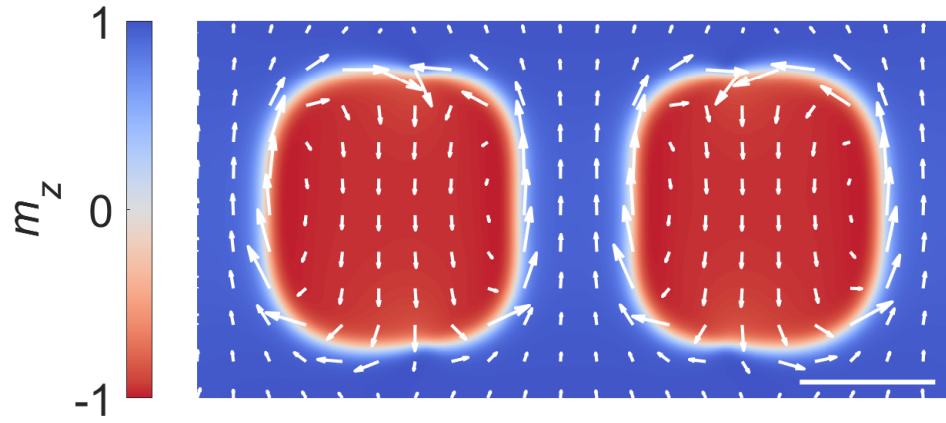

FIG. S2. Biskyrmions after removing the external field directly, in comparison with Fig.5(a) in the main text. The scale bar is 200 nm.
